# Supplementary material for: Generalizable task representation learning from human demonstration videos: a geometric approach
Source: arXiv:2202.13604 source file (2022-02-28)
Supplement: Supplementary file 1 [file supplementary.tex]

Each graph structure is derived by enumerating all possible node connections and filtering out graphs that do not satisfy the ``permutation-invariant'' or ``non-inner-associative'' property. To list all possible node connections inside a graph $\mathcal{G}$, we require any node $v \in \mathcal{G}$ that its degree should satisfy $deg(v) \geq 1$ and the intermediate connection nodes with $deg(v) \geq 2$, since the graph needs organize all the points without any node or edge isolations. For example, consider the line-to-line constraint using four keypoints. There are a total of 38 possible structures of $\mathcal{G}$. After filtering out, the structure shown in Fig. \ref{fig:c1} is selected out. Fig. \ref{fig:c2} shows the selection process.

\begin{figure}[h]
	\includegraphics[width=12cm]{raw/5/graph_structure_selection.pdf}
	\centering
	\caption[Select-out of graph structures.]{Examples of how the graph structure of point-to-line and line-to-line constraints are selected out. We firstly enumerate all possible node connections without any node or edge isolation, wherein the point-to-line has 4 candicates and the line-to-line has 38 candidates. Then we filter out candicates that violate the above mentioned two properties. As shown above, red dot indicates violation of the permutation-invariant property and yellow dot for the non-inner-associative property. To give examples of such violations, in B3, non-inner-associative property is violated since $g([x_{1}, x_{2}] , [x_{3}, x_{4}] )= g([x_{1}, x_{4}] , [x_{3}, x_{2}] )$.In B4, permutation-invariant property is violated since $g([x_{1}, x_{2}] , [x_{3}, x_{4}] ) \neq  g([x_{3}, x_{4}] , [x_{1}, x_{2}] )$. } 
	\label{fig:c2}
\end{figure}

\begin{figure}[]
	\includegraphics[width=0.99\textwidth]{raw/6/hammer_embedding_ll_single.pdf}
	\centering
	\caption[Visualize the task-specification correspondence]{Task-specification correspondence visualization of the hammering-LL task which involes two line parallelism to define the task. Results show our task function’s outputs that are the line-to-line constraint’s representation $z_{t}$ on categorical objects staying similar to each other while allowing individual varying factor changes. $z_{t}$ is visualized using 16 successive frames’ output and select the first component for visualization convenience. A complete visualziaton of all components of $z_{t}$ can be found in Fig. \ref{fig:a6_ll_details}.
	}
	\label{fig:6_task_embeddings_the_same2}
\end{figure}

\begin{figure*}
	\centering
	\includegraphics[width=1.0\textwidth]{raw/6/hammer_embedding_pp_whole_appendix.pdf}
	\caption[Visualize the task-specification correspondence]{Task-specification correspondence visualization of the hammering-PP task which involes two points coincidence to define the task. \textbf{Left:} the learned task function’s output $z_{t}$. For convenience, we visualize the first component of $z_{t}$ in 16 successive time steps.  Results show that the embedding $z_{t}$ for hammer A, B, C and D stays similar to each other while allowing slight value changes.  This is done by selecting image features on objects and construct a graph to represent their geometric constraints. $z_{t}$ is the representation of the constructed graph.  \textbf{Right:} a random selector's output $z_{t}$. Results show a random selector, though selects image features and constructs the same graph structure; the embedding $z_{t}$ of the four hammers do not match with each other. A complete visualziaton of all compooe
	}
	\label{fig:a6_pp_details}
\end{figure*}

\begin{figure*}
	\centering
	\includegraphics[width=1.0\textwidth]{raw/6/hammer_embedding_ll_whole_appendix.pdf}
	\caption[Visualize the task-specification correspondence]{Task-specification correspondence visualization of the hammering-LL task which involes two line parallelism to define the task. Again, results to the \textbf{left} are our task function’s outputs that show the line-to-line constraint’s representation $z_{t}$ on categorical objects stays similar to each other while allowing individual varying factor changes. \textbf{Right} shows the results using a random selector. $z_{t}$ is visualized using 16 successive frames’ output and select the first component for visualization convenience.
	}
	\label{fig:a6_ll_details}
\end{figure*}

\begin{figure}[h]
	
	\subfloat[Hammer A]{%
		\includegraphics[width=1.0\textwidth]{raw/9/hammer1_left.pdf}
	}
	\qquad
	\subfloat[Hammer B]{%
		\includegraphics[width=1.0\textwidth]{raw/9/hammer2.pdf}
	}
	\qquad
	\subfloat[Hammer C]{%
		\includegraphics[width=1.0\textwidth]{raw/9/hammer3.pdf}
	}
	\qquad
	\subfloat[Hammer D]{%
		\includegraphics[width=1.0\textwidth]{raw/9/hammer4.pdf}
	}
	
	\caption[Control curves of the hammering task]{Control curves of the hammering task by plugin the learned task function in a UVS controller. The task function was trained using human demonstrations of hammers A, B, and C. D is the new introduce hammer for testing.
	During UVS control, we use 4 joints in the task.	 \textbf{Left column}: image errors per time step when plugin the task function with the UVS controller. \textbf{Middle column:} joint velocity command from the UVS controller. The large joint velocity changes mostly happen when the estimation Jacobian matrix's condition number jumps high. This phenomenon also gives us the clue for future study of robust UVS. \textbf{Right column:} the Jacobian matrix's condition number per time step. During the experiment, the condition number of the estimated Jacobian remains low, which benefits from consistent geometric constraint selection and our normalized image errors described in Section 7.2.2.
	}
	\label{fig:8_UVS_control_tool_gen_hammer}
\end{figure}
